# Supplementary material for: On the Sample Complexity of Vanilla Model-Based Offline Reinforcement Learning with Dependent Samples
Source: arXiv:2303.04268 source file (2023-03-07)
Supplement: Supplementary file 1 [file appendix.tex]

\label{appendix}

In this section, we explain the derivation of Theorem \ref{thm:numberofrequiredpaths}.

 Lemma \ref{lemma:numberofsamplesfromsaq} provides an upper bound on the number of samples from a state-action pair, in order to estimate transition probabilities within a desired accuracy.

\begin{lemma} \label{lemma:numberofsamplesfromsaq}
 For any \(0 < \failureprob' < 1\) and \(\altstate \in \states \setminus \lbrace \deadstate \rbrace
 \),  if \[ \sum_{\altstate \in \states \setminus \lbrace \deadstate \rbrace} \numberofsampletransitions(\genericstate, \genericaction, \altstate) \geq 20 (\nicefrac{1}{\optimalitygap'})^{2} \log\left( \nicefrac{1}{\optimalitygap'} \right) \log \left(\nicefrac{5}{3 \failureprob'}\right)  , \] then \( |\hat{\probs}(\genericstate, \genericaction, \altstate) - \probs(\genericstate, \genericaction, \altstate)| \leq \optimalitygap' \) with probability at least \(1 - \failureprob'\).
\end{lemma}

Having identified the number of sample transitions required for a given state-action pair, our next goal is to determine the number of sample paths that ensures enough samples for the state-action pair. 
Lemma \ref{lemma:numberofpathswithsample} provides an upper bound on the number of sample paths that has a sample from a given state-action pair.
Lemma \ref{lemma:numberofsamplesperstateaction} provides an upper bound on the number of sample paths that has a sample from a given state-action pair, in order to ensure a desired number of sample transitions from the state-action pair. When Lemmas \ref{lemma:numberofpathswithsample} and \ref{lemma:numberofsamplesperstateaction} are combined, we get an upper bound on the number of sample paths to ensure enough samples for a given state-action pair.

\begin{lemma} \label{lemma:numberofpathswithsample}
Let \(\numberofpaths\) be the number of sample paths that are independently collected under \(\behaviorpolicy\). For any \(0 < \failureprob' < 1\), \(\numberofpaths' \geq 0\), and \((\genericstate, \genericaction) \in \states \times \actions\), if \[\numberofpaths \geq \max \left( \ceilx{\frac{2  \numberofpaths'}{\reachprob^{\behaviorpolicy}(\genericstate, \genericaction)}}, \ceilx{\frac{2 \log(\nicefrac{1}{\failureprob'})}{\reachprob^{\behaviorpolicy}(\genericstate, \genericaction)^2}} \right),\] then the number of sample paths that has a sample from \((\genericstate, \genericaction)\) is at least \(\numberofpaths'\) with probability at least \(1 - \failureprob'\).
\end{lemma}

\begin{lemma} \label{lemma:numberofsamplesperstateaction}
Let \(\numberofpaths'\) be the number of sample paths that has a sample from \((\genericstate, \genericaction) \in \states \times \actions \). For any \(0 < \failureprob' < 1\) and \(k \geq 0\),  if \[ \numberofpaths' \geq \max \left( \ceilx{k (1 - \loopprob^{\behaviorpolicy}(\genericstate,\genericaction))}, \ceilx{\frac{\log(\nicefrac{1}{\failureprob'})}{ \log(2) - \nicefrac{1}{2}}} \right), \] then the number of sample transitions from \((\genericstate, \genericaction)\) is at least \(k\) with probability at least \(1 - \failureprob'\).
\end{lemma}

%\frac{\cardstates^{4}  \maxreward^{2} \occupancymeasure^{\targetpolicy}(\genericstate, \genericaction)^{2}}{(1-\processcontinueprob)^2 \optimalitygap^{2}}
